# Supplementary material for: Defects from phonons: Atomic transport by concerted motion in simple crystalline metals
Source: arXiv:1912.01788 source file (2019-12-04)
Supplement: Supplementary file 1 [file supp.pdf]

# Supplementary Material:
# Defects from phonons:
# Atomic transport by concerted motion in simple crystalline materials

Erik Fransson and Paul Erhart[*]
*Chalmers University of Technology, Department of Physics, S-412 96 Gothenburg, Sweden*

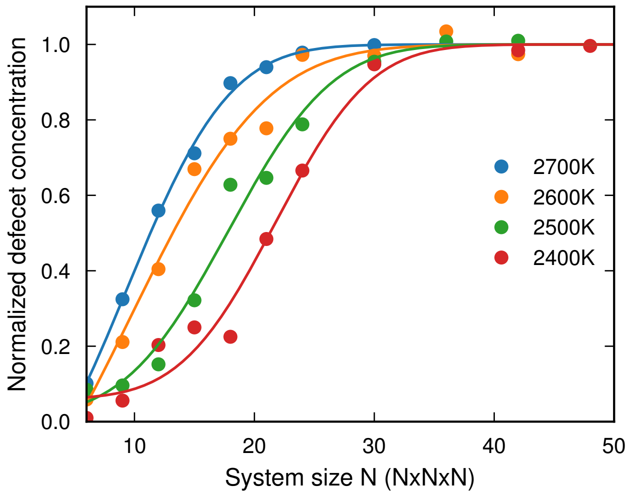


FIG. S1. Convergence of defect concentration in Nb with respect to system size and temperature. Defect concentrations are normalized for each temperature. $N$ indicates the number of conventional unit cells along each Cartesian direction. Solid lines serve as guides to the eye.

TABLE S1. Melting points, defect activation energies $E_A$, $\alpha = E_A/k_BT_m$, string barriers and BCC $\rightarrow \omega$ barriers as obtained using the empirical potentials used in this study.

| | $T_m$ (K) | $\alpha$ | $E_A$ (eV) | String barrier (eV) | BCC $\rightarrow \omega$ barrier (eV) |
|---|---|---|---|---|---|
| Ti | 1880 | 7.290 | 1.181 | 0.499 | 0.326 |
| Zr | 2097 | 13.641 | 2.465 | 0.843 | 0.468 |
| Ta | 3050 | 14.340 | 3.769 | 1.323 | 1.069 |
| Nb | 2680 | 16.632 | 3.841 | 1.108 | 1.048 |
| Mo | 3210 | 25.711 | 7.112 | 1.630 | 0.923 |
| W | 3708 | 23.497 | 7.508 | 2.036 | 1.545 |
| Cu | 1322 | 23.990 | 2.733 | 1.151 | |
| Al | 1041 | 24.993 | 2.242 | 1.010 | |
| Ni | 1726 | 23.048 | 3.428 | 1.241 | |

* erhart@chalmers.se

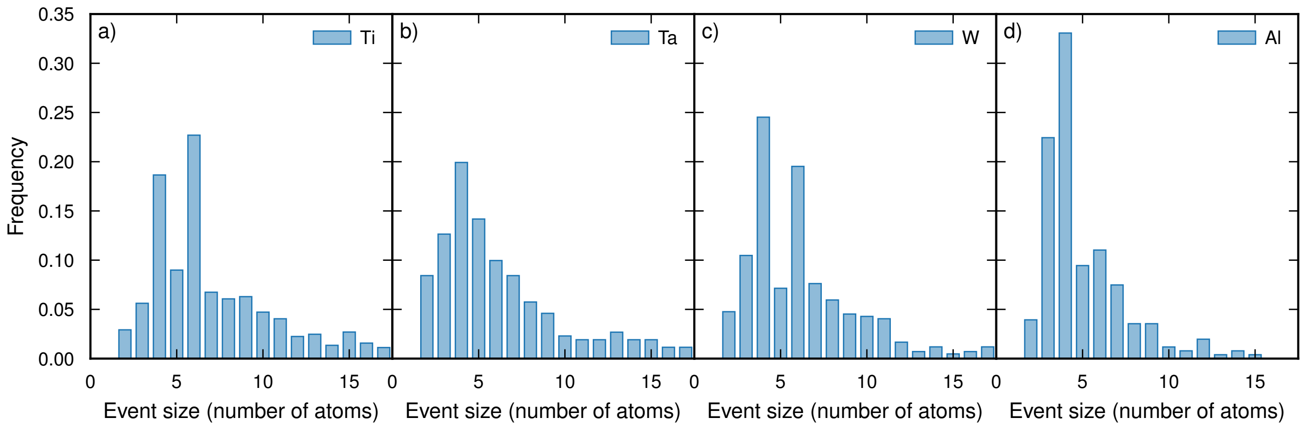


FIG. S2. Frequency of events by size for a) titanium, b) tantalum, c) tungsten, and d) aluminum.
